# Supplementary material for: COVIDHunter: An Accurate, Flexible, and Environment-Aware Open-Source COVID-19 Outbreak Simulation Model
Source: arXiv:2102.03667 source file (2022-06-08)
Supplement: Supplementary file 1 [file COVIDHunter_Bioinformatics-Supp-6Feb-Final.pdf]

*Supplementary Material for*  
**COVIDHunter: An Accurate, Flexible,  
and Environment-Aware Open-Source  
COVID-19 Outbreak Simulation Model**

Mohammed Alser, Jeremie S. Kim, Nour Almadhoun Alserr,  
Stefan W. Tell, and Onur Mutlu

*ETH Zurich, Zurich 8006, Switzerland*

## **1 Statistical Relationship Between Temperature and Number of COVID-19 Cases**

The purpose of this study is to explore the relationship between the daily new confirmed COVID-19 case counts or death counts and temperature in Switzerland. We obtain the daily number of confirmed COVID-19 cases and deaths in Switzerland from official reports of the Federal Office of Public Health (FOPH) in Switzerland [1] starting from March 2020 until January 2021. We obtain the air temperature data from the Federal Office of Meteorology and Climatology (MeteoSwiss) in Switzerland [2]. We calculate the daily average air temperature during the same time period (March 2020 to December 2020) for all the 26 cantons in Switzerland.

To evaluate the correlation between the temperature data and the number of daily confirmed COVID-19 cases or the daily counts of death, we use a generalized additive model (GAM). GAM is usually used to calculate the linear and non-linear regression models between meteorological factors (e.g., temperature, humidity) with COVID-19 infection and transmission [3, 4, 5]. Our analyses are performed with R software version 4.0.3., where  $p$ -value  $< 0.05$  is considered statistically significant. Our model attempts to represent the linear behavior of the growth curve of the counts of the new confirmed cases or deaths in Switzerland. Therefore, we can test the hypothesis of whether there is a significant negative correlation between the COVID-19 confirmed daily case or death counts and temperature.

The results demonstrate a significant negative correlation between temperature and COVID-19 daily case and death counts. Specifically, the relationship is linear for the average temperature in the range from 1-26°C. Based on Figure S1, we make two key observations. 1) For each 1°C rise in temperature, there is a 3.67% ( $t$ -value = 3.244 and  $p$ -value = 0.0013) decrease in the daily number of COVID-19 confirmed cases (Figure S1(a)). 2) For each 1°C rise in temperature, there is a 23.8% decrease in the daily number of COVID-19 deaths ( $t$ -value = 9.312 and  $p$ -value = 0.0), as shown in Figure S1(b).

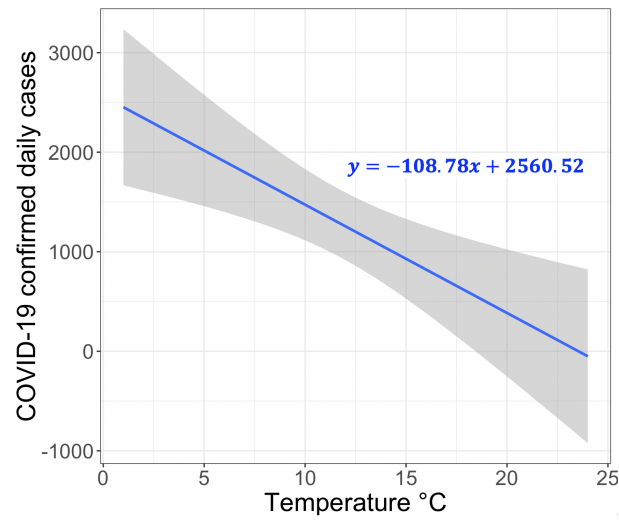

(a)

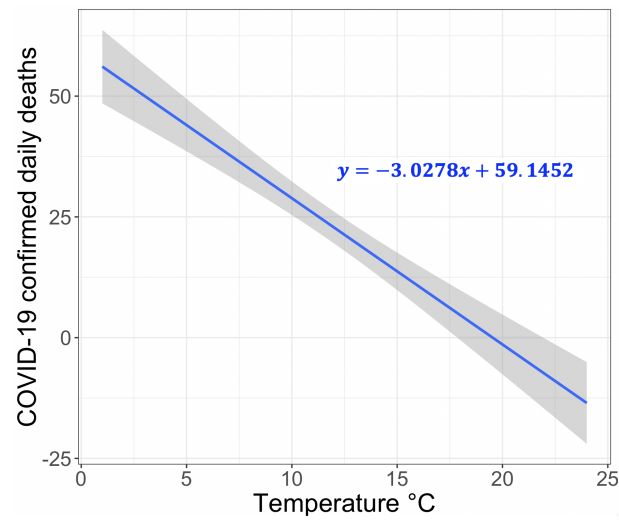

(b)

Figure S1: Correlation between temperature and COVID-19 confirmed (a) case count and (b) death count in 26 cantons of Switzerland.

## 2 Evaluating the Effect of Different Mitigation Coefficient Values on COVIDHunter’s Predicted Number of Cases, Hospitalizations, and Deaths

Using COVIDHunter, we predict the number of COVID-19 cases, hospitalizations, and deaths during 22 January to 31 March 2021. We show the maximum and the average of daily number of COVID-19 cases, hospitalizations, and deaths over 22 January to 31 March 2021 in Figures S2 and S3, respectively. We use two environmental condition approaches, CRW and CTC, with a certainty rate level of 50%. We assume five mitigation coefficient,  $M(t)$ , values of 0.35, 0.4, 0.5, 0.6, and 0.7 for each configuration of COVIDHunter during 22 January to 22 February 2021.

This range of mitigation coefficient values covers the lowest (i.e.,  $M(t)=0.35$ ) and the highest (i.e.,  $M(t)=0.7$ ) strengths of mitigation measures that have been applied during the year of 2020.

Based on Figures S2 and S3, we make three key observations. 1) COVIDHunter predicts that the *maximum* of daily number of COVID-19 cases, hospitalizations, and deaths over 22 January to 31 March 2021 would be 4972, 213, and 136, respectively, using CRW and  $M(t)=0.7$ , as we show in Figure S2(a-c). Using our environmental condition approach, CTC, and  $M(t)=0.7$ , the *maximum* of daily number of COVID-19 cases over 22 January to 31 March 2021 would be 7580 and the *maximum* of daily number of COVID-19 hospitalizations and deaths would be almost same as that calculated by COVIDHunter with CRW, as we show in Figure S2(d-f). 2) Relaxing the mitigation measures by 50% ( $M$  is changed from 0.7 to 0.35) *exponentially* increases the *maximum* of daily number of cases, hospitalizations, and deaths by  $58\times$ , reaching up to 288827, 12385, and 7885, respectively, as predicted by COVIDHunter with the CRW approach (Figure S2(a-c)). Using the CTC approach and  $M(t)=0.35$ , COVIDHunter predicts an *exponential* increase in the *maximum* of daily number of cases, hospitalizations, and deaths by *only*  $34.5\times$ , as we show in Figure S2(a-c). This is expected as the CTC approach considers only the drop in temperature rather than the average effect of many environmental conditions as the CRW approach does. 3) Relaxing the mitigation measures by 50% ( $M$  is changed from 0.7 to 0.35) causes the *daily* number of cases, hospitalizations, and deaths to *exponentially* increase by an average of  $29.6\times$  and  $23.8\times$  over 22 January to 31 March 2021 using CRW and CTC environmental approaches, respectively, as we show in Figure S3.

We conclude that COVIDHunter provides flexible evaluation of the effect of different strength of the past and current mitigation measures on the number of COVID-19 cases, hospitalizations, and deaths. COVIDHunter evaluates the applied mitigation measures with high flexibility of configuring the environmental coefficient and mitigation coefficient, which helps society and decision-makers to accurately review the current situation and estimate future impact of decisions.

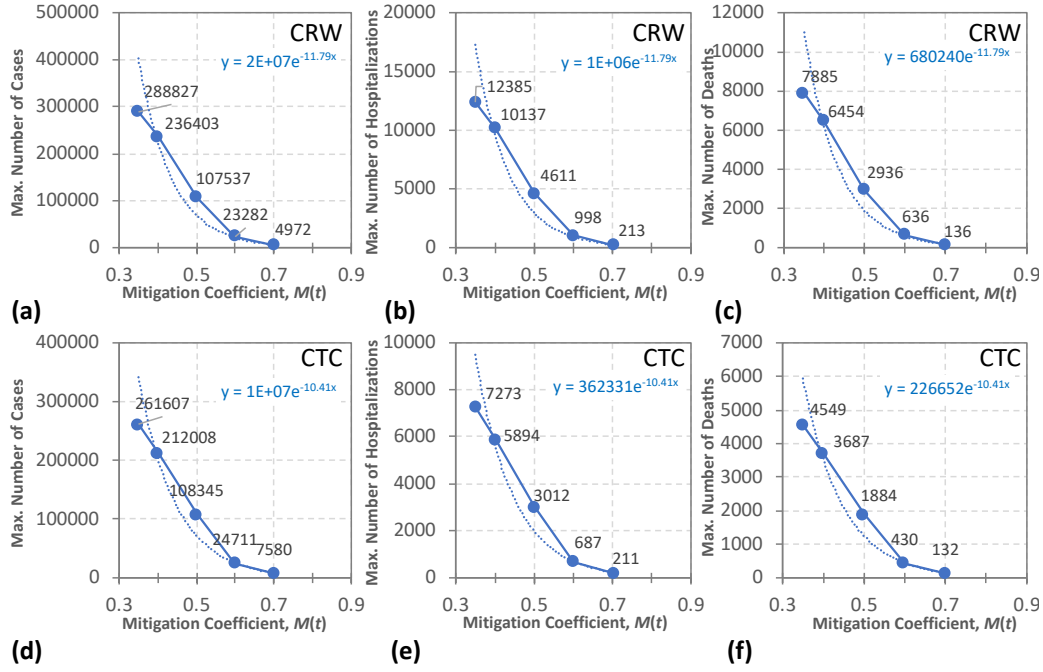

Figure S2: The maximum of daily number of COVID-19 cases, hospitalizations, and deaths as predicted by COVIDHunter over 22 January to 31 March 2021. We use five mitigation coefficient,  $M(t)$ , values of 0.35, 0.4, 0.5, 0.6, and 0.7 for each configuration of our model during 22 January to 22 February 2021. We use two different environmental condition approaches, CRW (a)-(c) and CTC (d)-(f) with a certainty rate level of 50%. Dashed line represents exponential model fit to data.

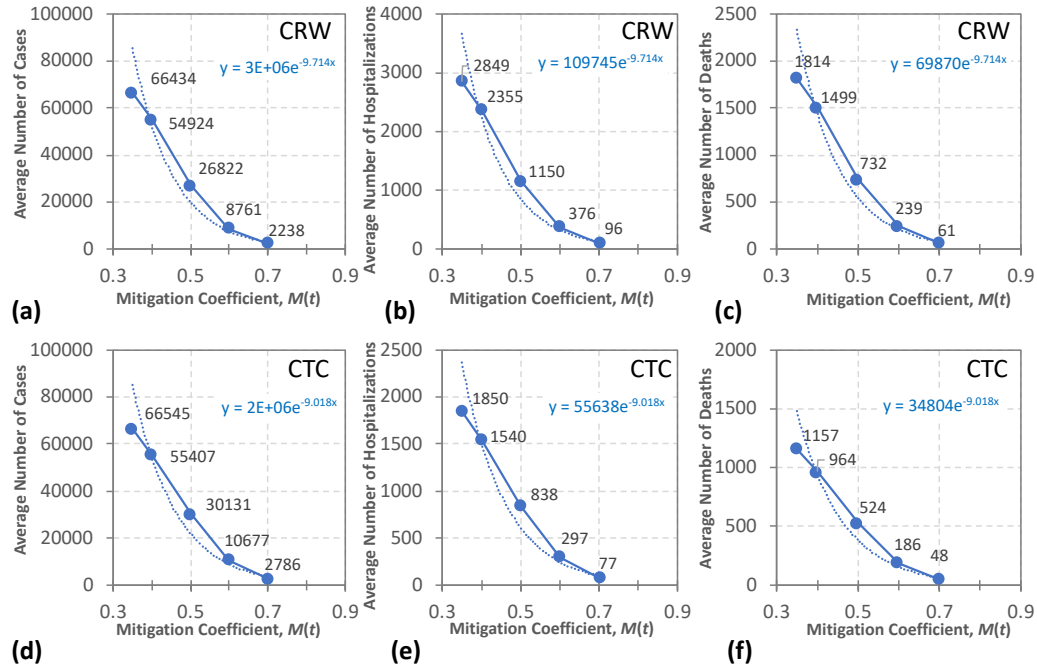

Figure S3: The average of daily number of COVID-19 cases, hospitalizations, and deaths as predicted by COVIDHunter over 22 January to 31 March 2021. We use five mitigation coefficient,  $M(t)$ , values of 0.35, 0.4, 0.5, 0.6, and 0.7 for each configuration of our model during 22 January to 22 February 2021. We use two different environmental condition approaches, CRW (a)-(c) and CTC (d)-(f) with a certainty rate level of 50%. Dashed line represents exponential model fit to data.

### 3 Evaluated Datasets

Our experimental evaluation uses a large number of different real datasets, including 1) daily  $R$  number values, 2) observed daily number of COVID-19 cases, 3) observed daily number of COVID-19 hospitalizations, 4) observed daily number of COVID-19 deaths, 5) number of excess deaths, 6) the estimated strength of mitigation measures as calculated by the Oxford Stringency Index, 7) estimation of COVID-19 statistics as calculated by existing state-of-the-art simulation models, ICL, IHME, LSHTM, and IBZ, from seven different sources as we list below. The raw datasets are provided in the [Supplementary Excel File<sup>1</sup>](#) and it can be also obtained from the original sources as we list below:

- Observed COVID-19 statistics (R number values and number of cases, hospitalizations, and deaths)
  - Official reports (January 7, 2021): <https://www.covid19.admin.ch/en/overview>
  - Smoothed data (January 7, 2021): <https://ourworldindata.org/coronavirus/country/switzerland?country=~CHE>
- Excess deaths:
  - Information: <https://www.bfs.admin.ch/bfs/en/home/statistics/health/state-health/mortality-causes-death.html>
  - Direct link (January 7, 2021): <https://www.bfs.admin.ch/bfs/en/home/statistics/health/state-health/mortality-causes-death.assetdetail.12607335.html>
- Oxford Stringency Index
  - <https://www.bsg.ox.ac.uk/research/research-projects/coronavirus-government-response-tracker#data>
- Imperial College London (ICL) Model:
  - Information: <https://mrc-ide.github.io/global-lmic-reports/>
  - Direct link (January 15, 2021): [https://github.com/mrc-ide/global-lmic-reports/raw/master/data/2021-01-30\\_v7.csv.zip](https://github.com/mrc-ide/global-lmic-reports/raw/master/data/2021-01-30_v7.csv.zip)
- Institute for Health Metrics and Evaluation (IHME) Model:
  - Information: <https://mrc-ide.github.io/global-lmic-reports/>
  - Direct link (January 15, 2021): <http://www.healthdata.org/covid/data-downloads>
- The London School of Hygiene & Tropical Medicine (LSHTM) Model:
  - Information: [https://cmmid.github.io/topics/covid19/global\\_cfr\\_estimates.html](https://cmmid.github.io/topics/covid19/global_cfr_estimates.html)
  - Direct link (January 15, 2021): [https://raw.githubusercontent.com/cmmid/cmmid.github.io/master/topics/covid19/reports/under\\_reporting\\_estimates/under\\_ascertained\\_estimates.csv](https://raw.githubusercontent.com/cmmid/cmmid.github.io/master/topics/covid19/reports/under_reporting_estimates/under_ascertained_estimates.csv)
- The Theoretical Biology Group at ETH Zurich (IBZ) Model:
  - Information: <https://ibz-shiny.ethz.ch/covid-19-re-international/>
  - Direct link (January 15, 2021): <https://github.com/covid-19-Re/dailyRe-Data>

### References

- [1] Coronavirus - The Federal Office of Public Health in Switzerland. <https://www.bag.admin.ch/bag/en/home/krankheiten/ausbrueche-epidemien-pandemien/aktuelle-ausbrueche-epidemien/novel-cov.html>. Accessed: 2020-12-31.
- [2] Switzerland forecast - The Federal Office of Meteorology and Climatology MeteoSwiss. <https://www.meteoswiss.admin.ch/home.html?tab=overview>. Accessed: 2020-12-31.

---

<sup>1</sup><https://github.com/CMU-SAFARI/COVIDHunter/blob/main/EvaluationResults/ComparisonToOtherModels.xlsx>

- [3] Jiangtao Liu, Ji Zhou, Jinxi Yao, Xiuxia Zhang, Lanyu Li, Xiaocheng Xu, Xiaotao He, Bo Wang, Shihua Fu, Tingting Niu, et al. Impact of meteorological factors on the COVID-19 transmission: A multi-city study in China. *Science of the Total Environment*, page 138513, 2020.
- [4] David N Prata, Waldecy Rodrigues, and Paulo H Bermejo. Temperature significantly changes COVID-19 transmission in (sub) tropical cities of Brazil. *Science of the Total Environment*, page 138862, 2020.
- [5] Jingui Xie and Yongjian Zhu. Association between ambient temperature and COVID-19 infection in 122 cities from China. *Science of the Total Environment*, 724:138201, 2020.
